# Supplementary material for: Catalecticant intersections and confinement of decompositions of forms
Source: arXiv:1911.07769 ancillary file (2020-05-27)
Supplement: Supplementary file 1 [file CatIntConf.pdf]

**ANCILLARY FILE TO  
“CATALECTICANT INTERSECTIONS AND CONFINEMENT  
OF DECOMPOSITIONS OF FORMS”**

ELENA ANGELINI, CRISTIANO BOCCI, LUCA CHIANTINI

The script of the algorithm mentioned in Remark 3.4 of the paper is the following:

```
k = QQ;
R = k[Z_0..Z_8];
a = for i from 1 to 2 list random 100
b = for i from 1 to 2 list random 100
c = for i from 1 to 2 list random 100
d = for i from 1 to 2 list random 100
e = for i from 1 to 2 list random 100
f = for i from 1 to 2 list random 100
Q1 = matrix{{1,0,0,0,0,0,0,0,0}};
Q2 = matrix{{0,0,0,0,1,0,0,0,0}};
Q3 = matrix{{0,0,0,0,0,0,0,0,1}};
Q4 = matrix{{1,1,1,1,1,1,1,1,1}};
Q5 = matrix{{a_0*d_0,a_0*e_0,a_0*f_0,b_0*d_0,b_0*e_0,b_0*f_0,c_0*d_0,c_0*e_0,c_0*f_0}};
Q6 = matrix{{a_1*d_1,a_1*e_1,a_1*f_1,b_1*d_1,b_1*e_1,b_1*f_1,c_1*d_1,c_1*e_1,c_1*f_1}};
A = Q1||Q2||Q3||Q4||Q5||Q6;
coe = gens(ker A);
P5 = ideal((vars R)*coe_{0},(vars R)*coe_{1},(vars R)*coe_{2});
B = transpose(genericMatrix(R,Z_0,3,3))
C = ideal(gens P5, gens minors(2,B));
dim C -- 2 (C defines an algebraic variety of affine dimension 2, i.e. an algebraic curve)
degree C -- 6 (C defines an algebraic curve of degree 6)
genus variety(C) --1 (arithmetic genus of the algebraic curve)
singularLocus(variety(C)) -- variety(ideal 1) (it's the empty set, i.e. the curve is smooth)
```

The script of the algorithm used in the proof of Proposition 4.1 part (i) of the paper is the following:

```
k = ZZ/31991;
S = k[s_0..s_2];
l = for i from 0 to 5 list random(1,S);
f1 = sum(6,i -> random(k)*(l_i)^3);
f2 = sum(6,i -> random(k)*(l_i)^3);
f3 = sum(6,i -> random(k)*(l_i)^3);
DD1 = diff(transpose vars(S),diff(basis(2,S),f1));
DD2 = diff(transpose vars(S),diff(basis(2,S),f2));
DD3 = diff(transpose vars(S),diff(basis(2,S),f3));
Cf = DD1||DD2||DD3;
rank Cf -- 6
```

Since we found that the matrix  $C_f$  has maximal rank over a finite field (of characteristic 31991), the same holds in characteristic 0.

In order to compute the degree of the curve  $\mathbb{P}(\text{im}(C_f)) \cap X_{1,1,1}^2$ , the previous script can be completed as follows:

```

--- we compute the cartesian equations of im C_f
kk = gens ker transpose Cf;
R = k[x_0..x_8];
kkk = sub(kk,R);
Image = ideal(vars(R)*kkk_{0}||vars(R)*kkk_{1}||vars(R)*kkk_{2});
dim Image -- 6
degree Image -- 1
-- we compute the cartesian equations of the affine cone over X_{1,1,1}^2
U = k[a_0..a_2,y_0..y_2];
a1 = matrix{{a_0,a_1,a_2}};
par1 = y_0*a1|y_1*a1|y_2*a1;
F = map(U,R,{par1_(0,0),par1_(0,1),par1_(0,2),par1_(0,3),par1_(0,4),par1_(0,5),par1_(0,6),
par1_(0,7),par1_(0,8)});
PAR1 = kernel F;
dim PAR1 -- 5
degree PAR1 -- 6
-- we compute the required intersection
INT = PAR1+Image;
dim INT -- 2 (INT defines an algebraic variety of affine dimension 2, i.e. an algebraic curve)
degree INT -- 6 (INT defines an algebraic curve of degree 6)
genus variety(INT) --1 (arithmetic genus of the algebraic curve)
singularLocus(variety(INT)) -- variety(ideal 1) (it's the empty set, i.e. the curve is smooth)

```

The computational verification of the equality  $\mathbb{P}(\text{im } C_f) = < [\ell_1^\vee \otimes (\lambda_1^1, \lambda_1^2, \lambda_1^3)], \dots, [\ell_6^\vee \otimes (\lambda_6^1, \lambda_6^2, \lambda_6^3)] >$  stated in Proposition 4.2, can be obtained as follows. To work with a general  $f$ , we assume that  $\ell_1 = x_0, \ell_2 = x_1, \ell_3 = x_2, \ell_4 = x_0 + x_1 + x_2$  and that  $\ell_5, \ell_6 \in \mathbb{C}[x_0, x_1, x_2]_1$  and  $\lambda_i^j$  are random elements. It suffices to show that the  $9 \times 12$  matrix  $C_f'$  obtained by juxtaposing to  $C_f$  the column vectors

- $(\lambda_1^1, 0, 0, \lambda_1^2, 0, 0, \lambda_1^3, 0, 0) \in [\ell_1^\vee \otimes (\lambda_1^1, \lambda_1^2, \lambda_1^3)] = [(1, 0, 0) \otimes (\lambda_1^1, \lambda_1^2, \lambda_1^3)]$
- $(0, \lambda_2^1, 0, 0, \lambda_2^2, 0, 0, \lambda_2^3, 0) \in [\ell_2^\vee \otimes (\lambda_2^1, \lambda_2^2, \lambda_2^3)] = [(0, 1, 0) \otimes (\lambda_2^1, \lambda_2^2, \lambda_2^3)]$
- $(0, 0, \lambda_3^1, 0, 0, \lambda_3^2, 0, 0, \lambda_3^3) \in [\ell_3^\vee \otimes (\lambda_3^1, \lambda_3^2, \lambda_3^3)] = [(0, 0, 1) \otimes (\lambda_3^1, \lambda_3^2, \lambda_3^3)]$
- $(\lambda_4^1, \lambda_4^1, \lambda_4^1, \lambda_4^2, \lambda_4^2, \lambda_4^2, \lambda_4^3, \lambda_4^3, \lambda_4^3) \in [\ell_4^\vee \otimes (\lambda_4^1, \lambda_4^2, \lambda_4^3)] = [(1, 1, 1) \otimes (\lambda_4^1, \lambda_4^2, \lambda_4^3)]$
- $(\lambda_5^1 \partial_{x_0} \ell_5, \lambda_5^1 \partial_{x_1} \ell_5, \lambda_5^1 \partial_{x_2} \ell_5, \lambda_5^2 \partial_{x_0} \ell_5, \lambda_5^2 \partial_{x_1} \ell_5, \lambda_5^2 \partial_{x_2} \ell_5, \lambda_5^3 \partial_{x_0} \ell_5, \lambda_5^3 \partial_{x_1} \ell_5, \lambda_5^3 \partial_{x_2} \ell_5) \in [\ell_5^\vee \otimes (\lambda_5^1, \lambda_5^2, \lambda_5^3)] = [(\partial_{x_0} \ell_5, \partial_{x_1} \ell_5, \partial_{x_2} \ell_5) \otimes (\lambda_5^1, \lambda_5^2, \lambda_5^3)]$
- $(\lambda_6^1 \partial_{x_0} \ell_6, \lambda_6^1 \partial_{x_1} \ell_6, \lambda_6^1 \partial_{x_2} \ell_6, \lambda_6^2 \partial_{x_0} \ell_6, \lambda_6^2 \partial_{x_1} \ell_6, \lambda_6^2 \partial_{x_2} \ell_6, \lambda_6^3 \partial_{x_0} \ell_6, \lambda_6^3 \partial_{x_1} \ell_6, \lambda_6^3 \partial_{x_2} \ell_6) \in [\ell_6^\vee \otimes (\lambda_6^1, \lambda_6^2, \lambda_6^3)] = [(\partial_{x_0} \ell_6, \partial_{x_1} \ell_6, \partial_{x_2} \ell_6) \otimes (\lambda_6^1, \lambda_6^2, \lambda_6^3)]$

has still rank 6. The corresponding script implemented in Macaulay2 is the following:

```

k = ZZ/31991;
S = k[x_0..x_2];
lambda = for i from 1 to 18 list random(k);
l5 = random(1,S);
l6 = random(1,S);
f1 = lambda_0*x_0^3+lambda_1*x_1^3+lambda_2*x_2^3+lambda_3*(x_0+x_1+x_2)^3+lambda_4*l5^3+
lambda_5*l6^3;

```

```
f2 = lambda_6*x_0^3+lambda_7*x_1^3+lambda_8*x_2^3+lambda_9*(x_0+x_1+x_2)^3+lambda_10*15^3+
lambda_11*16^3;
f3 = lambda_12*x_0^3+lambda_13*x_1^3+lambda_14*x_2^3+lambda_15*(x_0+x_1+x_2)^3+lambda_16*15^3+
lambda_17*16^3;
DD1 = diff(transpose vars(S),diff(basis(2,S),f1));
DD2 = diff(transpose vars(S),diff(basis(2,S),f2));
DD3 = diff(transpose vars(S),diff(basis(2,S),f3));
Cf = DD1||DD2||DD3;
rank Cf -- 6
L1 = transpose(matrix(S,{lambda_0,lambda_6,lambda_12}))*matrix(S,{1,0,0})
L2 = transpose(matrix(S,{lambda_1,lambda_7,lambda_13}))*matrix(S,{0,1,0})
L3 = transpose(matrix(S,{lambda_2,lambda_8,lambda_14}))*matrix(S,{0,0,1})
L4 = transpose(matrix(S,{lambda_3,lambda_9,lambda_15}))*matrix(S,{1,1,1})
L5 = transpose(matrix(S,{lambda_4,lambda_10,lambda_16}))*diff(vars S, 15)
L6 = transpose(matrix(S,{lambda_5,lambda_11,lambda_17}))*diff(vars S, 16)
Cf' = Cf|L1|L2|L3|L4|L5|L6
rank Cf' -- 6
```

The script of the algorithm used in the proof of Proposition 6.1 part (i) of the paper is the following:

```
k = ZZ/31991;
S = k[s_0..s_2];
l = for i from 0 to 9 list random(1,S);
f1 = sum(10,i -> random(k)*(l_i)^4);
f2 = sum(10,i -> random(k)*(l_i)^4);
f3 = sum(10,i -> random(k)*(l_i)^4);
f4 = sum(10,i -> random(k)*(l_i)^4);
DD1 = diff(transpose vars(S),diff(basis(3,S),f1));
DD2 = diff(transpose vars(S),diff(basis(3,S),f2));
DD3 = diff(transpose vars(S),diff(basis(3,S),f3));
DD4 = diff(transpose vars(S),diff(basis(3,S),f4));
Cf = DD1||DD2||DD3||DD4;
rank Cf -- 10
```

The list of 17 points obtained in Bertini via homotopy continuation and monodromy loops and mentioned in the proof of Proposition\* 6.4 is the following (in each row, the first value denotes the real part and the second one the imaginary part, both expressed in scientific notation; the square brackets identify the coordinates of each summand in a decomposition of  $\tilde{f}$ ):

```
1
[4.800622111180369e-02 1.646769768243992e-02
1.540400594032930e-01 1.047954693602667e-01
-2.042263016617713e+00 4.905681976636332e-01
-3.222184020270640e+00 1.197276545405050e+00]
[-9.033358972108502e-01 9.189605719320420e-01
7.158292650343849e-02 9.502672575916450e-01
-2.053431904544198e-01 -3.361949441459242e-01
-5.652040343825707e-01 2.610842096803470e-01]
[4.707731212064225e-01 1.412435663228921e+00
3.770440338352786e-01 -6.386461575513737e-01
-3.898969570335450e-02 -6.100621744922975e-03
2.778105907817183e-02 -2.827058310923789e-03]
[-1.786931810538363e-01 -6.318772525820919e-01
```

3.940745205930641e-01 -4.151878711646135e-01  
 -3.833585302878125e-01 4.583874718997340e-01  
 -3.124440868333855e-01 6.454072395059822e-01]  
 [1.864092100576789e-01 -6.413554412572526e-01  
 -5.922202966422702e-01 9.793489854032699e-01  
 6.004429751431962e-01 7.194858849610011e-01  
 -5.259443216052773e-01 6.591691757786580e-01]  
 [-1.578686591943005e-01 -5.696286555095625e-01  
 -6.712689949732528e-01 4.829579103627751e-01  
 9.784898206904376e-01 -6.976763926119168e-01  
 4.941499780643439e-01 -3.183151453279948e-01]  
 [-2.460419115923344e-02 -1.746854209805637e-01  
 -7.526918111783850e-01 -6.467907007092297e-01  
 1.233477517329253e-01 -6.262884152374604e-02  
 -1.397512001405760e-01 -9.248559946684201e-02]  
 [-4.602577743620752e-01 6.794780870336428e-01  
 6.854182672834309e-01 -2.662400813753935e-01  
 3.489822052072251e-01 -6.237479384396957e-02  
 -3.788313473303239e-01 -3.458600025243616e-01]  
 [-4.238415392276145e-01 -9.583231864102651e-02  
 6.118650933813862e-01 -9.106795086824246e-01  
 -7.927013596133431e-01 7.621229117278047e-01  
 -1.340518122908426e-01 5.902863924126454e-01]  
 [1.350081403202705e-01 4.460882470298024e-01  
 4.826832211010099e-01 1.842881980355610e-02  
 3.894897633983399e-01 1.493985042996462e+00  
 2.233192038903175e+00 -1.113890301938116e+00]

2

[-5.958773151147191e-02 1.305091704579748e-01  
 1.036247202151433e-01 5.568088145031603e-01  
 -1.014118280605673e-01 -1.276723769581559e-01  
 -1.193881840323766e+00 2.202055317623967e-01]  
 [-3.065857531696054e-01 -5.978686018222878e-02  
 4.796648437015763e-01 -1.101482692325643e+00  
 -9.705340608007295e-01 2.193320327208934e-02  
 -4.258291059336355e-01 1.058440646779845e-01]  
 [8.289806621585221e-01 -1.627696575022308e+00  
 -3.635736598033662e-01 2.425899514951118e+00  
 -2.267632677849853e-04 -1.892791385872212e-03  
 -2.876280905429474e-04 1.794310418456980e-03]  
 [7.438157405954403e-04 9.787405315188582e-01  
 4.665510510843785e-01 -2.045370153827548e-01  
 -3.831524758984308e-02 7.214484550367766e-01  
 7.177684333038328e-01 -6.629717638252943e-01]  
 [-9.493782595330509e-02 -2.472273119259437e-01  
 -2.526896606740947e-02 -5.705508156734139e-01  
 -1.356591831182182e+00 1.130868204839550e+00  
 -1.388485652075327e+00 1.376730148044688e+00]  
 [-9.830478253426448e-01 1.111400656057910e+00]

1.326704091515322e-01 9.858453727743933e-01  
 -8.370881996440317e-02 -2.294415779747501e-01  
 -4.142980634993073e-01 8.859690338725126e-02]  
 [2.224046225626432e-01 -6.381103568971056e-01  
 -6.976896018342154e-01 1.040962224688632e+00  
 7.149503360326779e-01 4.033826141913421e-01  
 -2.829619461834905e-01 5.357346416888975e-01]  
 [1.025111052194664e+00 2.107151544440588e-01  
 4.861327782260085e-01 7.518222052248484e-02  
 1.414811366178475e-02 2.801050727048902e-01  
 -2.989870488212339e-02 -6.266954379472114e-02]  
 [-4.688049114102696e-01 -4.565226320299148e-01  
 -5.324706198650219e-01 5.666216288195404e-01  
 7.808148456173699e-01 4.265698337955049e-01  
 4.242609116004254e-01 4.170243254735000e-02]  
 [9.395954969948379e-01 1.154936896647347e+00  
 3.710409168249968e-01 1.994133113974123e-01  
 1.897197904915761e-02 1.342732778567811e-01  
 7.032584927600891e-02 -1.651212696925647e-01]

3

[1.664073444538441e-01 -5.524259176456258e-01  
 -6.473024908997257e-01 9.369800382065036e-01  
 1.192819971701226e+00 5.606365917342178e-01  
 -2.875179749362903e-01 8.952041601566149e-01]  
 [-1.712557414696403e+00 -1.224187556116709e+00  
 8.307021301932092e-01 5.933200756263611e-02  
 2.151935760106229e-03 -8.231834866581456e-03  
 -9.890602955305930e-03 -1.785713831648874e-02]  
 [-2.904390800160600e-01 1.295536766512992e-03  
 8.894389072854342e-01 -3.892750456034238e+00  
 -4.367638013291708e-03 -4.297739093987838e-03  
 -4.513029480976894e-04 -6.375758636379344e-04]  
 [5.435423728415149e-02 7.312695654547127e-01  
 4.631890929082686e-01 -1.961243907784823e-01  
 -2.164492246003336e-01 1.255708727386265e+00  
 1.104208239825083e+00 -9.840711627491922e-01]  
 [-7.112489404106466e-02 3.424769184529050e-02  
 -3.015271277259693e-01 -6.276366016799981e-02  
 1.012388581086962e+00 2.415419701436367e-01  
 -1.066309776334227e+00 9.287316588092710e-02]  
 [-6.638037369541848e-01 9.479345395273304e-01  
 1.060108387876288e-01 1.137399188430039e+00  
 4.538885201483330e-01 4.914971486795586e-02  
 7.810066837553868e-02 -4.984737194466127e-01]  
 [6.863862713615163e-01 1.250828728427367e-01  
 8.870783415704334e-02 -3.348189551047612e-02  
 -4.084343680970596e-01 4.995414677465009e-01  
 -4.203593892402647e-02 1.485837178188784e-01]  
 [-3.176396158054730e-01 -2.116781400705714e-01]

2.908964107783965e-01 -6.803267294722095e-01  
 -2.151983296655875e+00 1.106892910609185e+00  
 -1.331899950547514e+00 1.223753694341716e+00]  
 [-7.149329040249424e-01 7.880607484147171e-01  
 1.600717490075549e-01 9.659164106105029e-01  
 -9.149421261455547e-01 -5.290452283205532e-01  
 -9.227533663677938e-01 9.677264911586851e-01]  
 [-1.688214132700441e-01 -8.737044892536250e-01  
 -5.058272085005536e-01 9.743574810768507e-02  
 1.302436831096556e-02 -4.123226648284822e-01  
 -4.473774199529257e-02 -3.472561777664454e-01]

4

[-3.224492910985111e-01 -6.261196801188106e-03  
 4.050595889752935e-01 -1.264127859744387e+00  
 -6.912787508247310e-01 -3.161232400308068e-01  
 -3.186531184705985e-01 -9.081201389417180e-02]  
 [-4.373268727359630e-01 -5.958908340809987e-01  
 -5.131481943480505e-01 5.270375576448312e-01  
 7.859476516042673e-01 5.347515283261767e-02  
 4.845133076532581e-01 -8.666589466298254e-02]  
 [-1.163392407990951e-01 -2.091302332444369e-01  
 -1.328371834555420e-02 -6.056551903266764e-01  
 -1.722810335492622e+00 1.432504286570000e+00  
 -1.568553802712089e+00 1.556097609715715e+00]  
 [6.277126878574070e-01 5.590860671864444e-01  
 3.240164082593284e-01 2.777908480528281e-02  
 5.481741175363670e-02 6.458524072307430e-01  
 3.666864440292458e-01 -1.800044707947509e-01]  
 [-1.003320386463763e+00 9.965962011143380e-01  
 6.564592716735385e-02 9.844376389707346e-01  
 -1.716042295532234e-01 -2.275628664876784e-01  
 -4.071582434067695e-01 2.236814568110404e-01]  
 [8.091613251945214e-02 7.728744715528083e-01  
 -1.900501811824905e+00 -2.653241086512057e+00  
 -5.600705347497369e-04 -2.900481273609788e-03  
 1.376973021563571e-04 -5.970490712249011e-04]  
 [-1.802211232689442e-01 1.960962493904585e-01  
 1.846123540069858e-01 5.048522062247685e-01  
 5.963035112890223e-02 -1.588445979006901e-01  
 -1.239766828383544e+00 -9.160054328410752e-02]  
 [2.290225378631259e-03 9.783663000132931e-01  
 4.832873186767686e-01 -2.521135663705255e-01  
 -9.176071765248978e-02 6.433646144254526e-01  
 6.103668397303704e-01 -5.155061511871786e-01]  
 [1.824522909982715e+00 -1.290694172110418e+00  
 4.966287047898961e-01 1.340032057562442e-01  
 -6.089316783119749e-03 -3.121064893855137e-04  
 -3.589082592968841e-03 -1.017740210261859e-02]  
 [1.564226935539351e-01 -6.364021458316741e-01

-6.153347509761517e-01 9.919559876586710e-01  
 7.618047298496092e-01 6.901207465015139e-01  
 -4.472709599569863e-01 6.754299136847238e-01]

5

[7.007740252824689e-02 -4.218545745636956e-01  
 2.205929909890920e-02 -4.560636248940888e-01  
 -8.935081836536354e-01 1.814305193320439e+00  
 -5.887723824121827e-01 2.199514704565577e+00]  
 [4.661086209783243e-01 4.432052759630542e-01  
 6.134000744904224e-01 -5.665183202131259e-01  
 -2.296811724650794e-01 -2.904128724095679e-01  
 6.290420237161033e-02 1.206411951070656e-01]  
 [-4.504698183344083e-01 8.823109000630632e-01  
 5.751515951430817e-01 -4.061666960693986e-01  
 2.933378824580190e-01 3.399589958331820e-02  
 -1.207886458723551e-01 -2.832053907676662e-01]  
 [-1.133277980759096e-01 5.068379307355102e-01  
 3.548041137277398e-01 8.541764588146517e-02  
 7.120249325398679e-01 8.331139812772226e-01  
 3.113760600407583e-01 -2.075209237208285e+00]  
 [-3.212670077671409e-01 -5.407589809144350e-02  
 5.810815856213413e-01 -1.003369205007349e+00  
 -9.648736666789933e-01 4.974158157132589e-01  
 -3.173230986507175e-01 3.512806431282390e-01]  
 [4.634594486047620e-01 -1.459754283287132e-01  
 7.872252167857324e-02 -3.341511961438061e-01  
 -1.749089747600388e+00 -7.396763812099266e-01  
 -1.423854192149502e+00 -2.655417034955041e-01]  
 [-1.144787170677266e-02 -6.817088910122536e-01  
 -4.635485221120674e-01 6.086791572172786e-01  
 3.908588577822279e-01 -1.909226035766718e+00  
 9.893524695595098e-01 -1.176100358436252e+00]  
 [-8.949367947700189e-01 8.212660706394965e-01  
 1.572906104372842e-02 8.943271548762291e-01  
 -3.676378679419923e-01 -3.568618500994949e-01  
 -5.988145959979413e-01 4.855001272868491e-01]  
 [2.788582826209288e-01 -1.963413319219414e-01  
 -6.325706554311497e-01 8.216661515252247e-02  
 1.686323974617102e-01 1.015407131497429e+00  
 -9.555342859157472e-02 3.539141551776814e-01]  
 [1.466024160215841e-01 -6.144833379666291e-01  
 -5.828836505077986e-01 8.288316236276022e-01  
 1.618033291593743e+00 1.861513033472197e+00  
 -7.418141351055311e-01 1.769051319856739e+00]

6

[-4.235011086136101e-01 3.335146228443543e-02  
 1.587337734082366e-01 2.303586781622684e+00  
 3.107437308942997e-02 -2.451812361588994e-02]

-5.906083935517334e-03 8.231200392028412e-04]  
 [8.868118131585852e-02 -4.912893075435542e-01  
 -6.607230788635052e-01 9.490761699109070e-01  
 1.370663903480730e+00 6.535236784920170e-01  
 -3.233956015591869e-01 8.601083212033011e-01]  
 [5.478144226730518e-02 7.209248533812858e-01  
 4.421418369840856e-01 -1.821592371179205e-01  
 -9.316840609894621e-02 1.401751771305880e+00  
 1.206436375848460e+00 -1.167314056898768e+00]  
 [1.867842447949033e-01 -4.226178688609946e+00  
 5.193397879901438e-01 1.576714443230512e+00  
 6.583433701028912e-05 -1.354362276050626e-04  
 7.144731420408812e-04 -1.127525027594011e-03]  
 [6.345726216758177e-02 -7.234382495459915e-01  
 -3.821442972500940e-01 -4.003567282319210e-01  
 -3.779644182924629e-01 -5.368672136523307e-02  
 -3.138641509913774e-01 9.834127523247338e-02]  
 [-3.292033981599279e-01 -1.421620126648298e-01  
 4.172952100685416e-01 -8.287442283862682e-01  
 -1.660168587924853e+00 7.636811943724058e-01  
 -8.190445157696065e-01 7.016727967962525e-01]  
 [9.455493741220239e-01 1.559527563293889e+00  
 -5.971759189619288e-01 1.000011336718826e+00  
 -7.012331767344568e-04 8.157081800083539e-03  
 3.456271554055178e-03 -1.772732855119778e-02]  
 [8.818055903184529e-01 9.592652962217844e-02  
 4.596127056392119e-02 -5.772594196208670e-02  
 -2.651629122275455e-01 3.055010738342252e-01  
 -6.127817982040494e-02 5.961367601637621e-03]  
 [-2.110040482685035e-02 -1.165472111298337e-02  
 -1.830852956021656e-01 -3.012463734090032e-01  
 4.594409075814004e-01 7.197068224996894e-02  
 -1.509919850903577e+00 4.272505339224479e-01]  
 [-8.980034363533594e-01 7.193768987026740e-01  
 7.144232460041011e-02 8.850024951939430e-01  
 -4.859827372725495e-01 -3.666712854676956e-01  
 -7.004864843728115e-01 5.718569508966892e-01]

7

[-8.283691048228672e-01 9.134301438912059e-01  
 1.009281279319696e-01 9.682890598832461e-01  
 -1.424602805037701e-01 -4.932810145791200e-01  
 -7.244549933181198e-01 1.122766738478379e-01]  
 [1.924540835196825e-01 -6.049970372684312e-01  
 -6.232042006877442e-01 9.238961965599065e-01  
 1.022432809394242e+00 7.281357221446781e-01  
 -3.955619950611012e-01 9.005710592759458e-01]  
 [-2.685887076520573e-01 8.719165605702498e-01  
 6.091025468135113e-01 7.567592384273498e-01  
 -1.616342489054151e-01 -1.611462669690986e-01]



-2.384889291659462e-01 7.405506512535952e-02]  
 [-2.174424778206183e+00 4.054883495909856e-01  
 7.304572626962487e-01 -4.610863903053621e-01  
 -5.692160994728792e-03 1.224467901613446e-03  
 -3.166243214933662e-04 1.295040508559014e-02]  
 [-3.116933845275822e-01 -7.726930818837979e-02  
 5.226384519936604e-01 -1.275812808211447e+00  
 -5.269981473514120e-01 -1.571323076010751e-02  
 -2.077219481057433e-01 1.882560499783473e-02]  
 [-8.856770555728034e-02 -8.341980286504137e-01  
 -6.386507119299728e-01 4.166715904699423e-01  
 1.396022434929444e-01 -5.209245601151690e-01  
 1.764200212715515e-01 -3.152325557459876e-01]  
 [-7.529132687729320e-02 8.374844007833711e-03  
 -1.800990719058738e-01 1.787815770863653e-01  
 1.466272080933338e+00 1.008239737033896e+00  
 -2.105518624876142e-01 -1.465166867867766e-01]  
 [6.341271165349730e-01 -1.914018963551590e-02  
 1.011320487138918e-01 -4.769017070557801e-02  
 -7.544070172384926e-01 2.092762433588470e-01  
 -2.311515546362180e-01 1.179897356373875e-01]  
 [-1.911749533545820e-01 -2.763842548263513e-01  
 6.810205899263722e-02 -5.635479196479089e-01  
 -1.744519247667767e+00 1.083502950930493e+00  
 -1.561952292771728e+00 1.422644897336862e+00]  
 [1.009016567381947e-01 7.657244167876568e-01  
 4.889730363658339e-01 -2.227622166759590e-01  
 -3.144993076634589e-01 9.202598664321228e-01  
 8.704924317884873e-01 -7.177187435596087e-01]

8

[-3.278220106361205e-01 -8.896217923387718e-02  
 5.784030608467889e-01 -9.935743166586480e-01  
 -9.705269501043434e-01 5.951544658905718e-01  
 -3.309825456310452e-01 4.068095863048693e-01]  
 [-3.793356350912029e-02 -2.372280661686315e-01  
 -1.219816926425258e-01 -4.738585485242854e-01  
 -1.190011884409867e+00 -2.133134319521329e-02  
 -1.604877429403476e+00 5.836154138337132e-01]  
 [-9.571310573587413e-01 8.956999391054792e-01  
 4.447395301812745e-02 9.688325095310719e-01  
 -2.454948015384293e-01 -2.887456026300261e-01  
 -4.906074841762296e-01 3.036045191704294e-01]  
 [5.697202436203319e-02 2.785882890725824e-01  
 7.569517673231989e-01 -4.366759347413562e-01  
 -3.997982419218855e-01 -1.809219268423996e-01  
 -2.285614022522038e-02 9.055940468864898e-02]  
 [-2.083443563874443e-01 -8.333317243537434e-01  
 -6.071771712251920e-01 4.585758092935225e-01  
 3.082317752992659e-01 -5.097788433122399e-01]

2.451278044137083e-01 -3.479231301929342e-01]  
 [1.611985518069718e-01 5.720086777396272e-01  
 3.806667423609476e-01 1.114764464451691e-01  
 7.884281787703366e-01 3.497093252747838e-01  
 1.036484996776108e+00 -1.388867469651972e+00]  
 [5.610559727818532e-02 1.362601999519472e-01  
 6.485262542299833e-02 2.291992026278771e-01  
 -8.054286508180173e-01 1.403511979583560e+00  
 -1.518447865695837e+00 1.341250409637221e+00]  
 [1.572770723696127e-01 -8.711852712135015e-01  
 1.840079833345422e-01 -7.250764580688714e-02  
 2.550158233717090e-01 1.365325690881483e-01  
 2.865140719572516e-01 1.452500928546835e-01]  
 [-1.920417635239232e-01 8.976053427731396e-01  
 5.068359979909094e-01 -3.533388149161308e-01  
 2.565882973937104e-01 5.225100546089545e-01  
 2.601322348978285e-01 -5.335035619024103e-01]  
 [1.779284195186793e-01 -6.266372721557812e-01  
 -6.324100285046909e-01 9.284464157886808e-01  
 9.810931774530010e-01 7.529332369120160e-01  
 -3.837753897210127e-01 8.790501904721956e-01]

9

[4.379907289792530e-01 3.363563477031028e-01  
 1.890306308283311e-01 -1.153327905220479e-02  
 2.432918083079456e-02 1.381437776376602e+00  
 6.245665427340396e-01 2.581677829073174e-01]  
 [-6.714432242596646e-02 -2.051284180571930e-01  
 -5.225967869112426e-01 -1.541241074223754e-01  
 2.630917223236255e-01 3.345342397746304e-01  
 -6.370704609199469e-01 -4.470104976596937e-01]  
 [-9.922240946230195e-01 -7.176610899376139e-01  
 4.517840614453620e-01 -3.737734048151703e-01  
 9.405267789523210e-02 -5.307356001865070e-02  
 5.822198070137592e-02 -1.454656649707119e-01]  
 [1.756534266865515e-01 -6.496265820516485e-01  
 -5.399597739965771e-01 9.346761797560949e-01  
 5.341780403645474e-01 1.057896476282459e+00  
 -7.309529763312869e-01 6.818537416131287e-01]  
 [-9.675422751062227e-01 9.481781293963725e-01  
 4.565850550527723e-02 9.727591120343555e-01  
 -1.905799650615503e-01 -2.549000922686666e-01  
 -4.160618776861351e-01 2.511946256790217e-01]  
 [-3.734728892690891e-01 -2.666872659389830e-01  
 3.372575228891194e-01 -6.492511631764173e-01  
 -2.041280405429002e+00 7.437544146623070e-01  
 -1.212712269771344e+00 1.206152624289547e+00]  
 [-1.081758164457185e-01 -6.256536540408512e-01  
 -6.271995132011412e-01 5.394701419565358e-01  
 1.023775377048267e+00 -9.941437632755731e-01]

5.578492381337800e-01 -1.359037510576436e-01]  
 [7.991202993792544e-02 8.256346907356816e-01  
 4.853701488407603e-01 -2.640149882640737e-01  
 -3.550533283807423e-01 8.573674668445751e-01  
 8.458733947285929e-01 -4.800267171000106e-01]  
 [-3.846215190392369e-01 -2.505575957224570e-02  
 1.246466549190592e+00 -1.061864425950895e+00  
 5.098738621461672e-02 1.447978356251737e-01  
 2.737857791288978e-02 2.770309461476454e-02]  
 [-3.022031023628470e-01 3.146684114929918e-01  
 1.199129913578173e-01 4.579815362691737e-01  
 -4.254039623103092e-01 -4.580968786247015e-01  
 -1.640379896309890e+00 2.631802168987242e-01]

10

[-2.064121890170753e-01 -6.313448131242559e-01  
 -6.667751759415562e-01 5.335773082489268e-01  
 8.039458254154567e-01 -4.535886559257249e-01  
 4.363248050408353e-01 -1.673633044606002e-01]  
 [2.082483220716952e-01 2.771084879283006e-01  
 3.018939673057273e-01 1.116009442487962e-01  
 7.450898983939501e-01 4.875468546011708e+00  
 6.968108445064569e+00 5.094999179152894e+00]  
 [1.197531796605615e-01 2.490029558601961e-01  
 2.847472698217784e-01 1.798646351830413e-01  
 -1.543004516412263e+00 -3.435225228785993e+00  
 -7.740662970808180e+00 -5.240748039005528e+00]  
 [-4.119089484457313e-01 -1.616476865605410e-01  
 5.353442635929508e-01 -8.696790760057174e-01  
 -1.076259017343921e+00 1.042210239633391e+00  
 -3.815020256461604e-01 8.545460690775503e-01]  
 [-7.338518078068327e-01 4.172640672514563e-01  
 5.579664280571460e-01 9.245983106567539e-02  
 -2.720747170896635e-02 -1.043919122361931e-01  
 -2.062076060768982e-01 3.189086545651940e-02]  
 [-1.175141457751519e-01 -2.045608061506419e-01  
 -3.207500703519300e-01 -7.026380699534690e-01  
 2.583657644480597e-02 6.506498314397970e-02  
 -3.843474919959226e-01 3.493126967977331e-01]  
 [-3.981489668558941e-01 -6.521840967216616e-01  
 4.849493603802612e-01 -4.532986081531771e-01  
 -4.173286258154899e-01 -1.016722687529762e-01  
 -4.887221604703773e-01 1.810494433976121e-02]  
 [-4.562727944241830e-02 9.298690378395014e-01  
 5.682555557873279e-01 -3.437579830721073e-01  
 -7.657950095000574e-03 4.848114787692521e-01  
 2.717944615094497e-01 -4.188958487249337e-01]  
 [-9.219401332983853e-01 9.241184732767535e-01  
 6.090343074576572e-02 9.612892488771484e-01  
 -2.094718457180251e-01 -3.098895352734179e-01]

-5.243010412795766e-01 2.612725717481211e-01]  
[1.988914839919547e-01 -6.432275103919467e-01  
-6.104777665625026e-01 9.625496855565702e-01  
6.841538503349337e-01 6.967862687941309e-01  
-4.737721621456650e-01 6.967263208329277e-01]

11

[-3.866508990761710e-01 -1.487241579227591e-01  
4.906702131711494e-01 -9.064398400008670e-01  
-1.279757975622620e+00 7.360717936329204e-01  
-6.016365750324070e-01 6.557108322114668e-01]  
[2.131301287786710e-01 -6.435477997878124e-01  
-6.210657610539748e-01 9.486272082516756e-01  
7.099457077886423e-01 6.655818102849236e-01  
-4.347516614945093e-01 7.147384667410484e-01]  
[-6.151559102589913e-01 4.610655307391354e-02  
3.777456743969809e-01 5.383600915165518e-01  
-4.417026680468831e-02 1.348467343351176e-01  
6.441825584721022e-03 2.410453999420848e-01]  
[1.490756873113313e-01 9.097235847754395e-02  
1.450692236118444e-01 2.321442608782449e-01  
-1.538987449677427e+00 2.467873169633434e-01  
-2.655585507991174e+00 4.817909006090859e-01]  
[-1.358003337759660e-01 -2.014312135810496e-01  
-2.375639815902192e-01 -6.412845600009588e-01  
-1.609183686720377e-01 1.684109809034368e-01  
-6.225909246548563e-01 5.641742565965932e-01]  
[2.605115634628610e-01 4.049723229237540e-01  
3.938087594338232e-01 1.270719577946905e-01  
7.925294362426644e-01 9.255196470969721e-01  
1.842575137133140e+00 -7.079363546551856e-01]  
[-9.105728710732275e-01 9.390674833286186e-01  
7.606271874559770e-02 9.662296349667171e-01  
-1.838432571761797e-01 -3.226282887688868e-01  
-5.380633263823960e-01 2.198074924212303e-01]  
[-9.125475219980464e-02 8.903872761485754e-01  
5.608595876533028e-01 -2.942345750598797e-01  
1.056339933061935e-01 5.992775713058861e-01  
3.104950997135018e-01 -5.963456862516507e-01]  
[-2.158083030110099e-01 -6.510218550229477e-01  
-6.809490939982384e-01 5.854654583871726e-01  
7.642707782908665e-01 -3.441850620199318e-01  
4.145213214093662e-01 -8.372901870817412e-02]  
[-4.436497051683943e-01 -8.024876597337968e-01  
4.959559704645385e-01 -4.320304245262051e-01  
-1.866058741799346e-01 -5.010858835562680e-02  
-2.446931350933104e-01 -9.410833692054541e-03]

12

[-1.033893114483894e-01 -2.237667653506994e-01

-5.074422274049544e-02 -4.957349741641990e-01  
 -1.879837266849160e+00 -4.243450124793521e-01  
 -1.593805472345125e+00 7.656113552190281e-01]  
 [-3.874953834796350e-01 -5.038075629178763e-02  
 5.864961853395223e-01 -1.021964771177624e+00  
 -7.802032935902299e-01 3.134477263191112e-01  
 -3.184759176850597e-01 2.883009710067141e-01]  
 [-2.961580065346138e-02 9.552830835569953e-01  
 4.923264638845123e-01 -3.253913510132350e-01  
 -1.072352316726064e-01 6.399266668546122e-01  
 5.494178684922386e-01 -3.241328996454823e-01]  
 [7.533067308758842e+00 -1.976909615020091e+00  
 2.195933603876721e+00 -2.298154446822588e+00  
 -7.505184704342385e-06 -2.875221226962913e-06  
 -2.355579779763365e-05 1.939641792217299e-05]  
 [7.260629733802756e-02 -6.190633975726471e-01  
 -7.595279744043779e-01 7.725805326318491e-01  
 1.402893331095833e+00 -4.141875607140920e-01  
 6.523378918842094e-01 5.630295590687748e-01]  
 [-8.438799890847600e-01 7.621485106136924e-01  
 3.510991184986802e-02 8.724288717143462e-01  
 -4.168059366649944e-01 -4.680738716524672e-01  
 -7.497541634629584e-01 5.508302197992875e-01]  
 [3.375530532664090e-01 6.313215924507262e-01  
 2.430272141522759e-01 -6.443214810524242e-02  
 5.194049090104268e-01 5.232384717063127e-01  
 8.060783422502195e-01 -3.567979754231602e-01]  
 [2.353849601809912e-01 -7.342338674382340e-01  
 -4.638301681296922e-01 8.453398190673599e-01  
 -2.790617273731691e-01 5.884315572620240e-01  
 -8.233597150393203e-01 -1.577769342591550e-03]  
 [2.410540891544014e-01 -5.907549883930171e-01  
 4.283839494926923e-01 -3.029755426188731e-01  
 3.642732877862965e-01 -5.174190809613492e-02  
 1.886549278376239e-01 1.620004024813678e-01]  
 [-9.328102004595992e-02 9.560267308217507e-02  
 3.243726021272871e-02 2.195250105022967e-01  
 1.546761569377881e-01 2.052880721399369e+00  
 -1.234357952941957e+00 -1.674378043674160e-01]

13

[5.007890651355131e-02 5.243664329593586e-01  
 1.514484311949530e-01 1.118332948447577e-01  
 5.716198364832401e-02 9.012966205218638e-01  
 2.482706662648109e+00 -4.139372377946167e-01]  
 [1.192755857722743e-01 -4.205482956138697e-01  
 3.049953800047603e-01 -3.296220535878381e-01  
 1.637847573082386e+00 4.826487971144875e-01  
 1.236984801206106e+00 7.205020080293315e-01]  
 [-3.988900022816594e-01 -1.772739367104833e-02]

6.061869843957465e-01 -1.035514321654958e+00  
 -7.324516261432034e-01 2.578928172527160e-01  
 -2.642952929519260e-01 2.768930902860680e-01]  
 [-1.430714625832811e-02 -5.880032392761111e-02  
 -7.626159378396374e-02 -3.948757078652269e-02  
 -6.474226427190735e-01 9.124993582012563e+00  
 -2.226307099899224e+00 3.130823836244083e+00]  
 [-4.241392408934003e-02 -1.544332648323530e-01  
 -1.565947263362506e-01 -2.854024086366690e-01  
 -2.428928644990074e+00 -7.277357981665932e+00  
 -2.064330361464388e+00 -2.622584582119230e+00]  
 [1.318461670927417e-01 1.373253840584393e+00  
 7.593386148747855e-01 5.952710670099652e-01  
 -8.461591364347394e-02 -7.304910158404397e-02  
 -1.735423358036233e-01 1.945744289042932e-01]  
 [2.478850370114289e-01 -6.629511589021975e-01  
 -5.282447173338570e-01 9.748218051557591e-01  
 3.255488436961089e-01 5.044497477760410e-01  
 -5.062122418926229e-01 4.337375427033155e-01]  
 [-1.379357698052091e-01 9.708285702571805e-01  
 5.327997125949638e-01 -3.963417999734854e-01  
 5.199613643759750e-02 4.284806610325780e-01  
 2.867206492165154e-01 -3.183165419260593e-01]  
 [1.669951151202958e-03 -5.094958730497603e-01  
 -8.990252127908823e-01 6.469525502943571e-01  
 8.103773801077674e-01 -6.063277119021585e-01  
 3.506148076241475e-01 6.762308374748074e-02]  
 [-5.973718760119517e-01 9.054614612733298e-01  
 1.880970307133264e-01 7.736257799519934e-01  
 -1.141636598087838e-02 -9.834535151799583e-01  
 -1.645627335491018e+00 1.052982713977846e-02]

14

[3.739160129159909e-01 5.247933846383946e-01  
 4.402786564461872e-01 -1.342926608525654e-02  
 3.736132788022118e-01 5.936107041223855e-01  
 1.005590495261438e+00 -4.675730647182955e-01]  
 [-8.662584720281662e-01 9.361101937064410e-01  
 1.193395925998520e-01 9.267423780083609e-01  
 -1.803739840907439e-01 -3.960675438991824e-01  
 -6.541272372218723e-01 1.909834474871272e-01]  
 [8.793897432374309e-02 9.685468697001516e-02  
 8.785551282297303e-02 2.010315237839712e-01  
 -1.110441946548951e+00 1.214899750243231e+00  
 -1.790565510959233e+00 7.271387649320014e-01]  
 [-2.239486310489119e-01 -1.605225153715580e-01  
 -2.707903072316367e-01 -5.566845941074760e-01  
 -3.089017285844721e-01 4.334561065061215e-02  
 -8.007682220110424e-01 3.356897584296997e-01]  
 [-3.821688268375881e-01 -1.153165386125826e-01

4.921159378025708e-01 -9.587090681063478e-01  
 -1.140325049633969e+00 4.913898249825676e-01  
 -5.197540204480221e-01 4.546082429033285e-01]  
 [-1.796708302426028e-01 -6.798811417131374e-01  
 -6.326354353020617e-01 4.216076596536007e-01  
 6.786032658310626e-01 -6.703691776329641e-01  
 4.231078835487607e-01 -3.769720287815041e-01]  
 [-1.683416689242942e-01 -8.841410664173940e-01  
 3.575390153823914e-01 -3.396261515558209e-01  
 -1.318983545534461e-01 1.823886831076172e-01  
 -1.511659104226434e-01 2.396573160023310e-01]  
 [-6.358718369852186e-02 9.253430679594681e-01  
 5.163150021417041e-01 -3.296382615985476e-01  
 -2.658016343628179e-02 5.613893484935136e-01  
 4.214298493167107e-01 -4.255816459571248e-01]  
 [1.932872491487622e-01 -6.269146556543713e-01  
 -6.104468476286992e-01 9.395817731911041e-01  
 8.223256496057876e-01 7.366075805132215e-01  
 -4.591782829747611e-01 8.027706134670887e-01]  
 [1.931527198700367e-02 -1.653388403496987e+00  
 -1.848690556731875e+00 -1.106577284163508e+00  
 2.075756104280713e-03 2.379134797154831e-03  
 2.143209102738414e-03 -8.759485502068105e-04]

15

[-8.334904141969557e-01 9.616326308383588e-01  
 1.077343924742033e-01 8.747362183625287e-01  
 -1.293178417031369e-01 -4.248108399676511e-01  
 -7.060576376440551e-01 1.372860462939708e-01]  
 [6.716671098606236e-01 4.506047725697545e-01  
 3.301983758690606e-01 -8.783669218182658e-02  
 1.534183816046703e-02 6.962979090673201e-01  
 3.018376510774483e-01 -7.856633987877346e-02]  
 [-1.193149666327163e-01 1.867025053885583e-01  
 5.803307714466941e-02 4.639532339812202e-01  
 2.121668573799268e-01 -4.537674195006157e-02  
 -1.518824256558724e+00 3.251671479354243e-01]  
 [-3.323562022146230e-01 -8.643518902857875e-02  
 6.127288987782676e-01 -1.072634370427366e+00  
 -7.244028346884275e-01 3.397195983283494e-01  
 -2.681312999642896e-01 2.333035335184231e-01]  
 [4.384130703087166e-02 -1.040585653738014e+00  
 -2.016107600419855e-01 7.009578693096977e-01  
 -8.728155030858847e-02 -1.736628109792703e-01  
 5.043089872313510e-03 -3.024748059673687e-01]  
 [1.669108722894885e-01 9.704643641780473e-01  
 4.925799623043073e-01 -2.734889251690037e-01  
 -3.208744879277183e-01 5.520346223878500e-01  
 6.798276918137078e-01 -3.293265152324647e-01]  
 [-4.186708912127160e+00 8.120063497874176e-01

1.950511788637131e-01 -1.119404218891009e-01  
 -2.973234285128192e-04 -2.995091581229189e-04  
 -1.860928702490327e-03 9.107694777479550e-04]  
 [-1.579200615011645e-01 -3.345081044665188e-01  
 -1.117795119990121e-02 -5.280804927127526e-01  
 -1.418561293652793e+00 5.140169414623586e-01  
 -1.435314859417474e+00 9.850597260100652e-01]  
 [1.283124346663358e-01 -5.882446132097283e-01  
 -6.979396984078248e-01 9.008540032078345e-01  
 1.316599099597598e+00 4.114062676457002e-01  
 -5.092555184911811e-02 8.931543348687284e-01]  
 [-4.006591344039687e-01 3.771544902476537e-02  
 -3.659039397036753e-01 4.804141966980262e-01  
 1.147242600666661e-01 8.902484785416828e-01  
 4.711183545647561e-01 -3.846684418113083e-01]

16

[-3.012966641169989e-01 -9.856009025609727e-02  
 4.330547428417874e-01 -1.032604187727969e+00  
 -1.203856583299084e+00 1.306142744411004e-01  
 -5.642780513787152e-01 1.629509170196142e-01]  
 [-2.559492057833517e-01 -7.190644442603798e-02  
 -2.418073117651800e-01 6.724353118881682e-01  
 9.666186136254714e-01 6.871516922378994e-01  
 -9.217046794562990e-02 1.225775789635176e-01]  
 [7.871410110777001e-01 2.155674184045070e-01  
 7.115242027390387e-01 -6.233821250758324e-01  
 -1.081260777961364e-01 -5.095167989362379e-02  
 -4.458975501304465e-02 3.812097774547506e-02]  
 [7.910341340341215e-01 -3.837899534468692e-01  
 -1.769799612493226e-01 3.952397281420651e-02  
 -3.700691489101131e-01 -8.810314238106820e-02  
 -1.607942634591482e-01 -1.605670317593683e-01]  
 [-1.818836861330538e-02 7.397898120465927e-01  
 4.632369462093268e-01 -1.190644123978259e-01  
 3.110011190319163e-01 1.039732625772838e+00  
 7.003129088593060e-01 -1.362041908132563e+00]  
 [-8.725335443758367e-01 7.811989045251904e-01  
 2.940314401648920e-02 9.206173827230190e-01  
 -4.029286456456807e-01 -4.256219947801994e-01  
 -6.854802698489437e-01 4.763334086798384e-01]  
 [-2.387622907779639e-01 -1.192372588467200e+00  
 -1.067502145093860e+00 7.214656508237247e-01  
 1.172838844954208e-01 -9.284440834057504e-02  
 9.306311685584759e-02 -2.556978511475204e-02]  
 [2.789726984425951e-01 -6.648762949851651e-01  
 -6.286290360464037e-01 9.179502346447795e-01  
 7.210975178033015e-01 6.131691097466224e-01  
 -3.840069484895383e-01 7.398805781623604e-01]  
 [-2.061207165132397e+00 2.798147040624195e+00



7.185812920840315e-01 -1.222540003844490e+00  
 6.235062468629206e-04 1.269036462126229e-04  
 -3.985052734292799e-04 -1.411287230947848e-03]  
 [-4.692100873396177e-02 -2.293965703329265e-01  
 -6.269494588448589e-02 -5.494126970624234e-01  
 -1.053547462056478e+00 9.463005349289492e-01  
 -1.384945511114631e+00 1.489572006881271e+00]

17

[-2.973122698788781e+00 -4.457298409325383e+00  
 4.065883461173133e+00 1.041447457053076e+01  
 4.283570427341069e-06 -2.685083550947811e-06  
 -1.962876325908696e-06 -1.938883442633134e-07]  
 [-2.420523172007537e-01 4.870594832975016e-01  
 2.048302125832403e-01 9.167853591069812e-02  
 1.707602462577319e+00 7.767446515148712e-01  
 -2.450246802418194e-02 -2.743218115415078e+00]  
 [7.798759475890380e-03 -5.602123015587494e-01  
 -6.010705179262119e-01 8.025037787506107e-01  
 1.914436355236122e+00 3.864013000067878e-01  
 4.523725714744881e-01 1.126030021470529e+00]  
 [2.864766208834247e-01 1.254404939418279e-01  
 5.451454591551969e-01 -2.697032309944567e-01  
 -5.106153379436104e-01 -9.814225313957781e-01  
 5.710637390276618e-01 -3.191065553389587e-01]  
 [3.030668546366121e-01 -7.352211509659626e-01  
 -1.029542058850690e-02 -6.512249752711831e-01  
 9.199704278088600e-02 2.995757748627768e-01  
 2.321862358168381e-01 4.170727153110478e-01]  
 [-2.099464223283784e-01 1.102570324848313e+00  
 6.580452939611098e-01 -6.821485021017149e-01  
 5.168840326614736e-02 1.590568480914184e-01  
 6.678733798526011e-02 -1.221745867163007e-01]  
 [1.263002827318390e-01 -8.284303730974080e-01  
 -3.490643329044935e-01 1.009547098127139e+00  
 -3.343526841763054e-01 1.496432228243225e-01  
 -4.766952241547790e-01 -3.563007692867514e-01]  
 [3.072592691386063e-01 -4.196076626974306e-02  
 1.275811198780713e-01 -2.837339670116926e-01  
 -1.771154418248224e+00 1.520097262684776e+00  
 -2.111724158484958e+00 2.007034150894263e+00]  
 [-3.005949909500092e-01 -7.275365045049510e-02  
 5.105054263654822e-01 -8.542785966960989e-01  
 -1.586433187373119e+00 8.537833563407968e-01  
 -5.503203162822865e-01 6.566821893657078e-01]  
 [-8.574489462733205e-01 7.437618858922469e-01  
 -1.248228243334537e-02 8.134472372848703e-01  
 -5.850761961941636e-01 -4.043032844682636e-01  
 -6.824535012896428e-01 8.138265988183310e-01]

The script of the algorithm mentioned in Example 7.2 and constructed via Macaulay2 to show that, for generic choice of a plane sextic, the investigated catalecticant map has rank 9, is the following:

```
k = ZZ/31991;
S = k[s_0..s_2];
l = for i from 0 to 8 list random(1,S);
f = sum(9,i -> random(k)*(l_i)^6);
Cf = diff(transpose basis(3,S),diff(basis(3,S),f));
rank Cf -- 9
```

In order to compute the degree of the curve  $C_9 = \mathbb{P}(\text{im}(C_f)) \cap X_3^2$ , the previous script can be completed as follows:

```
-- we compute the cartesian equations of im C_f
kk = gens ker transpose Cf;
R = k[x_0..x_9];
kkk = sub(kk,R);
Image = ideal(vars(R)*kkk_{0});
dim Image --9
degree Image --1
-- we compute the cartesian equations of the affine cone over X_{3}^2
U = k[a_0..a_2];
a3 = symmetricPower(3,matrix{{a_0,a_1,a_2}});
par1 = a3;
F = map(U,R,{par1_(0,0),par1_(0,1),par1_(0,2),par1_(0,3),par1_(0,4),par1_(0,5),par1_(0,6),
par1_(0,7),par1_(0,8),par1_(0,9)});
time PAR1 = kernel F
dim PAR1 -- 3
degree PAR1 -- 9
-- we compute the required intersection
INT = PAR1+Image;
dim INT -- 2 (INT defines an algebraic variety of affine dimension 2, i.e. an algebraic curve)
degree INT -- 9 (INT defines an algebraic curve of degree 9)
genus variety(INT) --1 (arithmetic genus of the algebraic curve)
```

The computational verification of the equality  $\mathbb{P}(\text{im}(C_f)) = \langle \nu_3([\ell_1^\vee]), \dots, \nu_3([\ell_9^\vee]) \rangle$  can be obtained as follows:

```
k = ZZ/31991;
S = k[s_0..s_2];
l = for i from 1 to 9 list random(k);
m = for i from 0 to 8 list random(1,S);
f = sum(9,i -> l_i*(m_i)^6);
Cf = diff(transpose basis(3,S),diff(basis(3,S),f));
rank Cf -- 9
L1 = diff(transpose basis(3,S),l_0*(m_0)^3);
L2 = diff(transpose basis(3,S),l_1*(m_1)^3);
L3 = diff(transpose basis(3,S),l_2*(m_2)^3);
L4 = diff(transpose basis(3,S),l_3*(m_3)^3);
L5 = diff(transpose basis(3,S),l_4*(m_4)^3);
L6 = diff(transpose basis(3,S),l_5*(m_5)^3);
L7 = diff(transpose basis(3,S),l_6*(m_6)^3);
L8 = diff(transpose basis(3,S),l_7*(m_7)^3);
L9 = diff(transpose basis(3,S),l_8*(m_8)^3);
```

```
Cf' = Cf|L1|L2|L3|L4|L5|L6|L7|L8|L9;  
rank Cf' --9
```

(E. Angelini, C. Bocci, L. Chiantini) DIPARTIMENTO DI INGEGNERIA DELL'INFORMAZIONE E SCIENZE MATEMATICHE,  
UNIVERSITÀ DI SIENA, VIA ROMA 56, 53100 SIENA, ITALIA

*E-mail address:* [elena.angelini@unisi.it](mailto:elena.angelini@unisi.it), [cristiano.bocci@unisi.it](mailto:cristiano.bocci@unisi.it), [luca.chiantini@unisi.it](mailto:luca.chiantini@unisi.it)
